# Supplementary material for: Learning Visual Robotic Control Efficiently with Contrastive Pre-training and Data Augmentation
Source: arXiv:2012.07975 source file (2022-10-17)
Supplement: Supplementary file 1 [file appendix.tex]

\section{Appendix}
\subsection{Task Description}
\label{appendix:tasks}
\label{sec:task_details_short}

For all of our real robot tasks, the reward function is the same as the discrete reward in Fetch suite, with $0$ when the task is in a completion state, and $-1$ everywhere else. 
% Since policy evaluation requires a task success function (usually done via human labeling), using this function as reward signal is feasible for how fast \ferm trains.
By design, our experiments are easy to reset at completion states, by simple hard-coded procedures.
Our assumptions allow \ferm to simply run with very little supervision, where the only human supervision is the 10 collected demonstrations.
% To speed up learning on the real robot, the episode length is shortened to 30 steps, rather than the default 50 in the Fetch suite. The normalized reward is computed by adding the episode length to the reward, and dividing by the episode length.

\begin{enumerate}
    \item \textbf{Reach}:
    The Robot must move to the block location. We consider a success when the gripper camera view has the block in its center. 
    The gripper is constrained to be unable to reach low enough to interact with the block. The gripper aperture is locked to a set position.
    During training, we fix the block location, however the demonstrations include random block locations.
    The arm is reset to a random location after every episode.
    \item \textbf{Pickup}:
    Success is declared if the robot picks the block up a specified height (70mm) above the work surface.
    At the end of each episode, if the gripper is around the block, it will reset the block to a random position, as well, resetting the gripper to a random location.
    \item \textbf{Move}:
    An episode is deemed successful when the block is moved to the center, onto the goal. Specifically, reward is given when the goal and the block are close while both visible from the griper camera.
    This task is especially difficult, as the block can be anywhere relative to the goal, so the system must understand to move the block in many directions, rather than a generic direction.
    As with Pickup, the block is reset at the end of each episode if the gripper can close and pick the block to a random location.
    \item \textbf{Pull}:
    The gripper aperture is locked at a set position.
    Without gripping onto the sponge, the robot must pull the sponge to an area around its base.
    At the end of each successful episode, the sponge is moved to a new random position.
    \item \textbf{Light switch}:
    A light switch panel is fixed to the work surface, and a blue LED lights up when the switch is flipped on.
    The gripper aperture is locked at a set position.
    Reward is given when blue light is visible from the gripper camera. At the end of each episode, a hard-coded reset procedure is executed to turn off the light. 
    \item \textbf{Drawer open}:
    The drawer is fixed to the work surface. The robot must grab onto the handle to pull open the drawer. Success is declared when the handle is visible from the gripper camera while the gripper position corresponds to the drawer being open. The drawer is closed by a hard-coded reset procedure at the end of each episode.
    
\end{enumerate}

For Reach, Light switch, and Drawer open tasks, the goal is fixed, and so the reset is hard-coded. 
For Pickup and Move, the block is only reset to a random location when the gripper is gripping the block, and for Pull, the sponge is only reset upon successfully pulling the sponge to the base of the robot.
% Although we used resets, the resets are only used upon success (near-success for Pickup and Move). 
% Our reward function is a less constrictive version than other RL methods, such as dense rewards, or Reward Sketching. 
\subsection{Qualitative Analysis \& Baselines}

\begin{wrapfigure}{r}{0.35\textwidth}
    \vspace{-2mm}
    % \centering
    \includegraphics[height=3.3cm, trim={20px 0px 20px 10px}, clip]{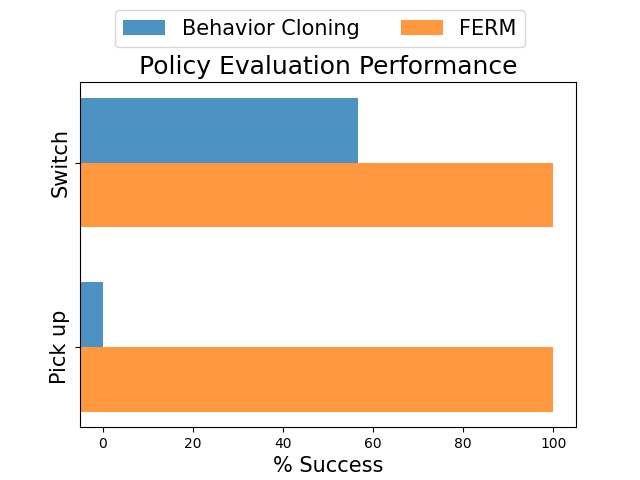}
    % \includegraphics[height=3.2cm]{figures/baselines/pickup.png}
    % \includegraphics[height=3.2cm, trim={10px 0px 40px 20px}, clip]{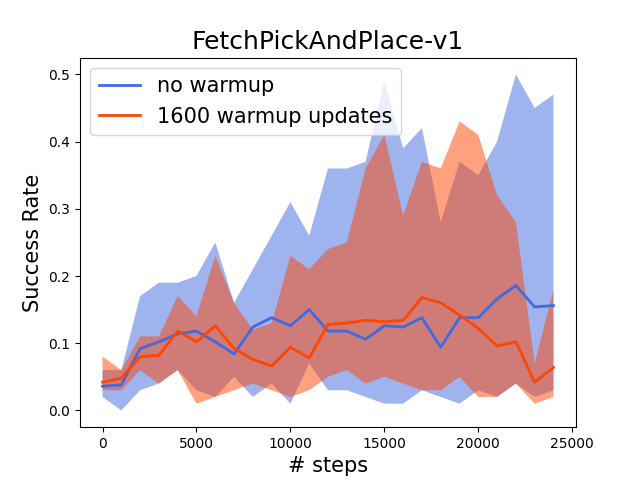}
    % \includegraphics[height=3.2cm, trim={10px 0px 40px 20px}, clip]{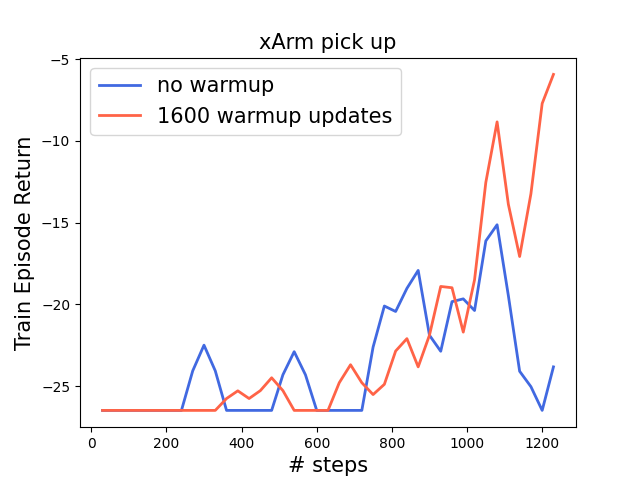}
%   \caption{Behavior cloning behavior on the Light Switch and Pickup task. Using the same demonstrations as our method, behavior cloning has limited capabilities due to low amounts of demonstrations.}
% \label{fig:baselines}
% \vspace{-6mm}
    % \vspace{5pt}
    % \includegraphics[height=3.2cm, trim={10px 0px 40px 20px}, clip]{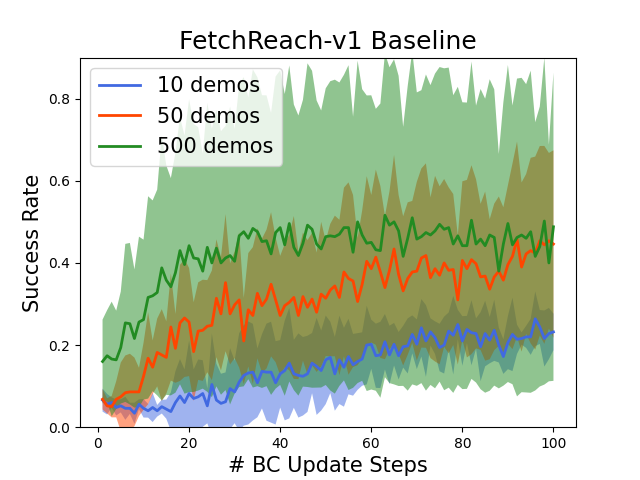}
    % \includegraphics[height=3.2cm, trim={10px 0px 40px 20px}, clip]{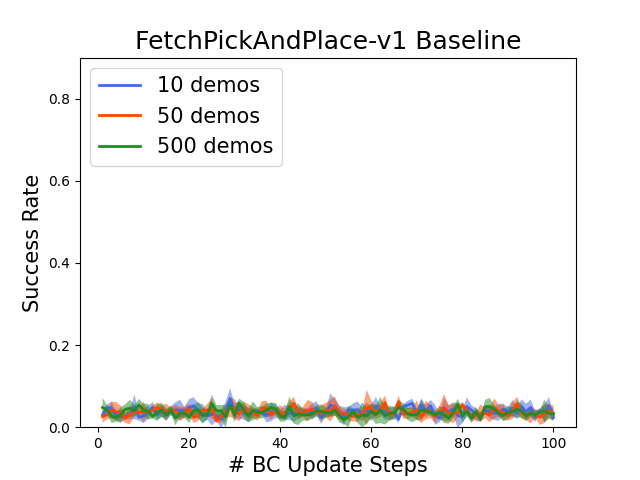}
    % \includegraphics[height=3.2cm, trim={10px 0px 40px 20px}, clip]{figures/ablation_warmup_pnp.png}
    % \includegraphics[height=3.2cm, trim={10px 0px 40px 20px}, clip]{figures/ablation_warmup_pick.png}
%   \caption{In simulation, the Behavior cloning baseline is only able to recover a sub-optimal policy for the Reach task.}

    \caption{Reported are the success rates on the Light Switch and Pickup task from Figure 5.}
    % \ferm is able to complete the task on every evaluation.}
\label{fig:baselines}
\vspace{-3mm}
\end{wrapfigure}

For our real world experiments, we qualitatively examine the policies learnt using \ferm versus behavior cloning from the same 10 demonstrations on a random goal (pickup), and a fixed goal task (switch). 
Videos of the policies are on the project website\footnote{\url{https://sites.google.com/view/efficient-visual-robotics}}, as well as the video in the Supplementary Materials.
% For the light switch task, even though the light switch remained stationary during training and demonstrations, the \ferm policy generalizes, and is able to complete the task even when the switch is moved to a never before seen location. 

We found that behavior cloning was able to complete the task around half of the time (17/30 trials) at the same position,
as the policy learned to memorize the steps necessary to flip the switch at the specified position. The most frequent failure mode occurred when the policy did performed the movement to flip the switch, but missed the actual switch. When the switch was moved from the training and demonstration location, this failure was inevitable every time. 
In contrast, the \ferm policy generalizes, and is able to complete the task even when the switch is moved to a never before seen location.

For the Pickup task, the policy trained with \ferm has intrinsic robustness to perturbation and generalization.
When the block is poked with a stick, the policy is able to recover even when the block is poked out from the gripper.
As well, the policy generalizes to pick up similarly colored blocks with different shapes.

The pickup policy learnt through behavior cloning was unable to locate the block at all, due to the low amount of demonstrations.
Even with lucky resets near the block, the policy is not robust to interactions with the block and fails to pick the block up.
\subsection{Further Ablations}
\label{sec:further_ablations}

\subsection{Demonstrations}

We perform the same experiment from Figure 7 with the FetchReach, and FetchSlide. 

\subsubsection{Camera setup}

\label{sec:ablation_camera}

In our experiments, we find that within the two-camera setup, the gripper-mount egocentric camera provides strong signals to the policies. We ablate the effect of camera placement to justify our final camera configuration. Shown in Figure \ref{fig:abalation_cams}, the egocentric view is crucial for the PickAndPlace task, as it alone is able to achieve decent results. However, taking frames from both cameras still proves advantageous, as the over the shoulder camera provides guide in direction when the object or the goal is outside the view of the gripper mount camera. For push, both cameras are needed for the agent to learn a meaningful control policy.

\subsubsection{Unsupervised Pre-training}

In simulation, we noticed that the unsupervised pre-training had no significant benefit in performance within the first $50$ episodes of training. In real world experiments, warming up the encoder has a significant difference on low environment step regimes, as seen in Figure~\ref{fig:ablation_unsupervised}. 
We hypothesize that contrastive pre-training enables fast learning, by accelerating the process of learning the relevant features from the environment observations. Since real world features are more difficult to extract, the real world experiments benefit more from the unsupervised pre-training.
To further test this hypothesis of accelerating feature extraction to aid the RL agent, we train \ferm, except we pre-train the encoders on the CIFAR-10 dataset \cite{CIFAR}, under the MIT License with the same contrastive loss. 
The performance at a low amount of environment steps is indistinguishable, and asymptotic performance is worse.
Figure~\ref{fig:further_ablation_unsupervised} summarizes our results for the PickAndPlace task in simulation.
As our hypothesis would suggest, learning \textit{incorrect} features from the CIFAR-10 dataset impedes learning, and hurts asymptotic performance.

\begin{figure}[h!]
    \centering
    \begin{subfigure}{0.48 \textwidth}
        \centering 
        \includegraphics[width=0.48\textwidth, trim={10px 0px 40px 20px}, clip]{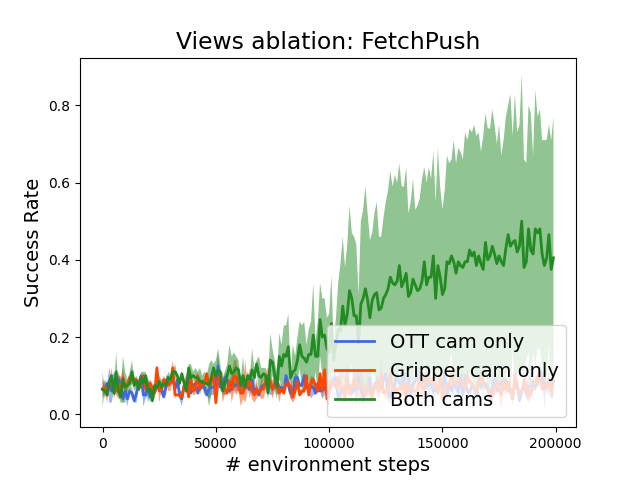}
        \includegraphics[width=0.48\textwidth, trim={10px 0px 40px 20px}, clip]{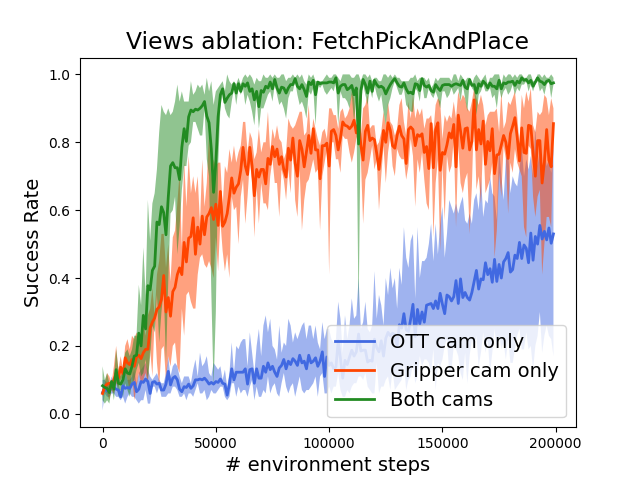}
        \subcaption{Camera setup ablation}
        \label{fig:abalation_cams}
    \end{subfigure}
    \begin{subfigure}{0.48 \textwidth}
        \centering 
        \includegraphics[width=0.48\textwidth, trim={10px 0px 40px 20px}, clip]{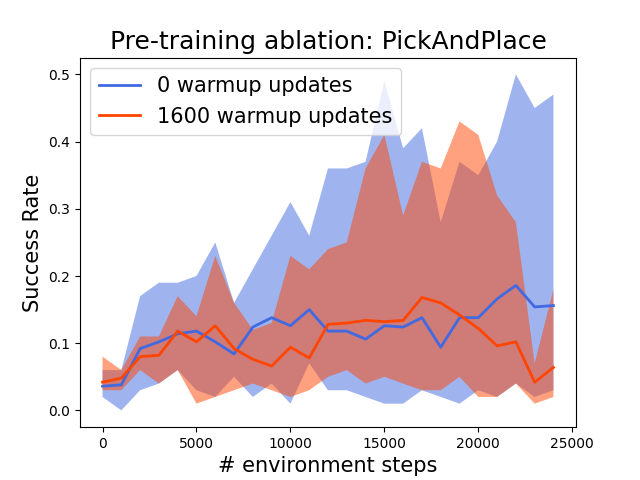}
        \includegraphics[width=0.48\textwidth, trim={10px 0px 40px 20px}, clip]{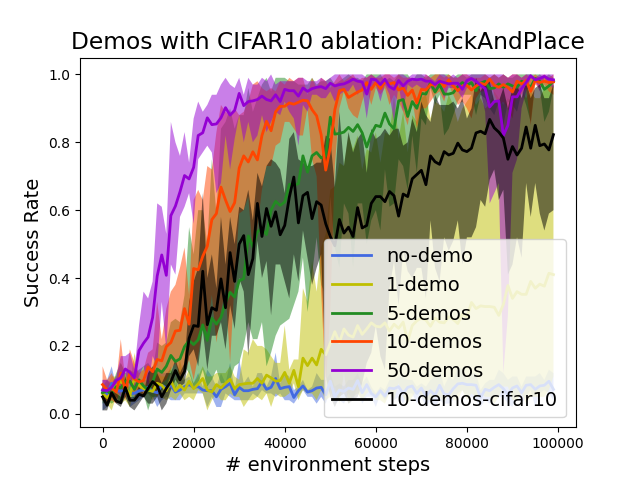}
        \subcaption{Unsupervised pre-training ablation}
        \label{fig:further_ablation_unsupervised}
    \end{subfigure}
    \caption{(a) Camera setup ablation: we compare the policy performance when trained with either one of RGB images or both. The use of both cameras proves essential for both the Push and PickAndPlace task. (b) Unsupervised pretraining ablation: \textbf{Left}: In the PickAndPlace task, warming up the encoder does not introduce significant difference to the RL training performance at low amounts of environment steps. \textbf{Right}: When the contrastive pre-training is done on an out of distribution dataset, \ferm is unable to achieve the same performance as pre-training with the demonstration observations.}
    % \caption{Camera setup ablation: we compare the policy performance when trained with either one of RGB images or both. The use of both cameras proves essential for both the push and pick-and-place task.}
    % \label{fig:further_ablation_unsupervised}
\end{figure}
