# Supplementary material for: Learning Visual Robotic Control Efficiently with Contrastive Pre-training and Data Augmentation
Source: arXiv:2012.07975 source file (2022-10-17)
Supplement: Supplementary file 2 [file ablations_appendix.tex]

\subsection{Further Ablations}
\label{sec:further_ablations}

\subsection{Demonstrations}

We perform the same experiment from Figure 7 with the FetchReach, and FetchSlide. 

\subsubsection{Camera setup}

\label{sec:ablation_camera}

In our experiments, we find that within the two-camera setup, the gripper-mount egocentric camera provides strong signals to the policies. We ablate the effect of camera placement to justify our final camera configuration. Shown in Figure \ref{fig:abalation_cams}, the egocentric view is crucial for the PickAndPlace task, as it alone is able to achieve decent results. However, taking frames from both cameras still proves advantageous, as the over the shoulder camera provides guide in direction when the object or the goal is outside the view of the gripper mount camera. For push, both cameras are needed for the agent to learn a meaningful control policy.

\subsubsection{Unsupervised Pre-training}

In simulation, we noticed that the unsupervised pre-training had no significant benefit in performance within the first $50$ episodes of training. In real world experiments, warming up the encoder has a significant difference on low environment step regimes, as seen in Figure~\ref{fig:ablation_unsupervised}. 
We hypothesize that contrastive pre-training enables fast learning, by accelerating the process of learning the relevant features from the environment observations. Since real world features are more difficult to extract, the real world experiments benefit more from the unsupervised pre-training.
To further test this hypothesis of accelerating feature extraction to aid the RL agent, we train \ferm, except we pre-train the encoders on the CIFAR-10 dataset \cite{CIFAR}, under the MIT License with the same contrastive loss. 
The performance at a low amount of environment steps is indistinguishable, and asymptotic performance is worse.
Figure~\ref{fig:further_ablation_unsupervised} summarizes our results for the PickAndPlace task in simulation.
As our hypothesis would suggest, learning \textit{incorrect} features from the CIFAR-10 dataset impedes learning, and hurts asymptotic performance.

\begin{figure}[h!]
    \centering
    \begin{subfigure}{0.48 \textwidth}
        \centering 
        \includegraphics[width=0.48\textwidth, trim={10px 0px 40px 20px}, clip]{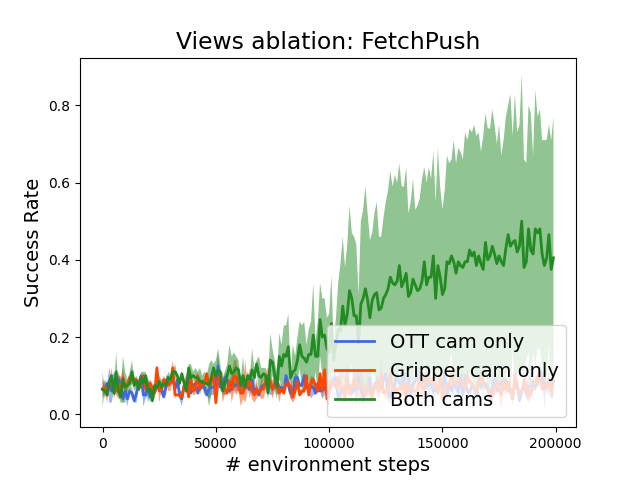}
        \includegraphics[width=0.48\textwidth, trim={10px 0px 40px 20px}, clip]{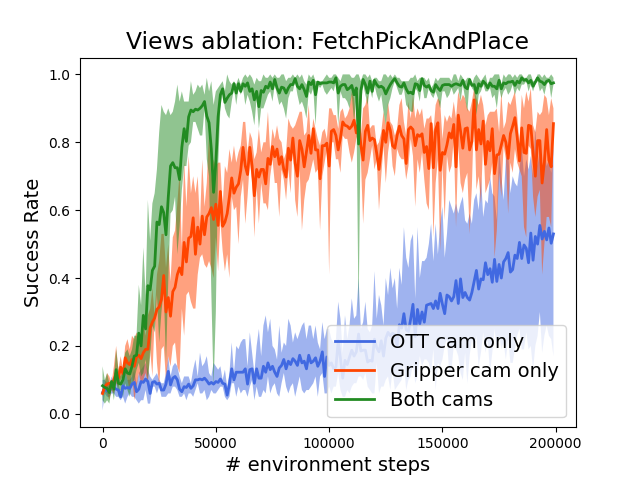}
        \subcaption{Camera setup ablation}
        \label{fig:abalation_cams}
    \end{subfigure}
    \begin{subfigure}{0.48 \textwidth}
        \centering 
        \includegraphics[width=0.48\textwidth, trim={10px 0px 40px 20px}, clip]{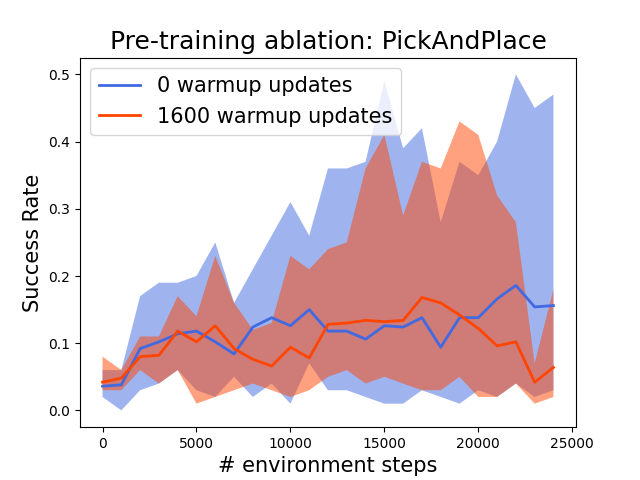}
        \includegraphics[width=0.48\textwidth, trim={10px 0px 40px 20px}, clip]{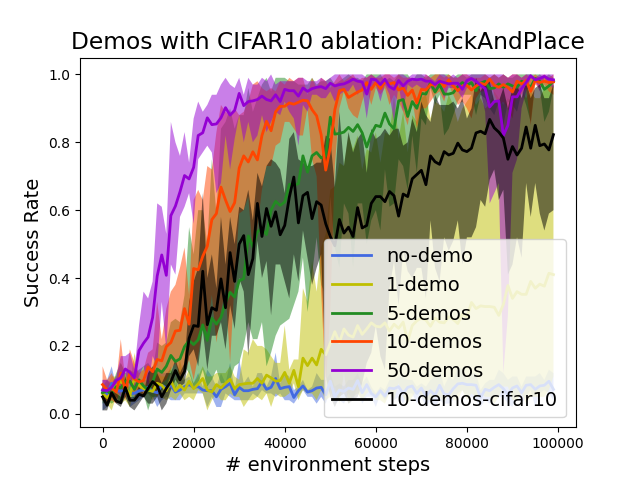}
        \subcaption{Unsupervised pre-training ablation}
        \label{fig:further_ablation_unsupervised}
    \end{subfigure}
    \caption{(a) Camera setup ablation: we compare the policy performance when trained with either one of RGB images or both. The use of both cameras proves essential for both the Push and PickAndPlace task. (b) Unsupervised pretraining ablation: \textbf{Left}: In the PickAndPlace task, warming up the encoder does not introduce significant difference to the RL training performance at low amounts of environment steps. \textbf{Right}: When the contrastive pre-training is done on an out of distribution dataset, \ferm is unable to achieve the same performance as pre-training with the demonstration observations.}
    % \caption{Camera setup ablation: we compare the policy performance when trained with either one of RGB images or both. The use of both cameras proves essential for both the push and pick-and-place task.}
    % \label{fig:further_ablation_unsupervised}
\end{figure}
